# Supplementary material for: Scaling Law for Time-Reversal-Odd Nonlinear Transport
Source: arXiv:2311.01219 source file (2024-12-09)
Supplement: Supplementary file 1 [file supp.pdf]

# Supplemental Material for "Scaling Law for Time-Reversal-Odd Nonlinear Transport"

Yue-Xin Huang,[1] Cong Xiao,[2,*] Shengyuan A. Yang,[2,†] and Xiao Li[1,‡]

[1] Department of Physics, City University of Hong Kong, Kowloon, Hong Kong, China

[2] Institute of Applied Physics and Materials Engineering, University of Macau, Taipa, Macau, China

## CONTENTS

I. Scaling law and physical mechanisms for ZOE contribution 1

II. Solution of ZOE terms from Boltzmann equation 4

III. Transverse ZOE conductivities in Dirac model 7

References 7

## I. SCALING LAW AND PHYSICAL MECHANISMS FOR ZOE CONTRIBUTION

In the main text, we have described our approach to derive the general scaling law for $\mathcal{T}$-odd nonlinear conductivity. Essentially, following the procedure in [1], the distribution function in the first and second order of applied electric field can be obtained from a set of linear equations.

For the $E$-linear corrections $f^{(1,j)}$ $(j=0,1,2)$, one has

$$\hat{\mathcal{I}}_{\rm c}^{(0,-2)} f^{(1,2)} = \hat{\mathcal{D}}_{\rm E} f_0, \tag{S1}$$

$$\hat{\mathcal{I}}_{\rm c}^{(0,-2)} f^{(1,1)} = -\hat{\mathcal{I}}_{\rm sk}^{(0,-3)} f^{(1,2)}, \tag{S2}$$

$$\hat{\mathcal{I}}_{\rm c}^{(0,-2)} f^{(1,0)} = -\hat{\mathcal{I}}_{\rm sj}^{(1,-2)} f_0 - \hat{\mathcal{I}}_{\rm sk}^{(0,-3)} f^{(1,1)} - \hat{\mathcal{I}}_{\rm sk}^{(0,-4)} f^{(1,2)}, \tag{S3}$$

$$\hat{\mathcal{I}}_{\rm c}^{(0,-2)} f^{(1,\text{-}1)} = -\hat{\mathcal{I}}_{\rm sk}^{(0,-3)} f^{(1,0)} - \hat{\mathcal{I}}_{\rm sk}^{(0,-4)} f^{(1,1)}, \tag{S4}$$

$$\hat{\mathcal{I}}_{\rm c}^{(0,-2)} f^{(1,\text{-}2)} = -\hat{\mathcal{I}}_{\rm sk}^{(0,-3)} f^{(1,\text{-}1)} - \hat{\mathcal{I}}_{\rm sk}^{(0,-4)} f^{(1,0)}, \tag{S5}$$

where we suppress the subscript $l$ for $f$. In each equation, the $(E, V^{-1})$ order is balanced on the two sides. Equations (S1-S3) have been obtained by Sinitsyn *et al.* before and found successful application in the study of linear AHE [2, 3].

These equations have a nice structure, which allows $f^{(1,j)}$ to be solved one by one in descending order of $j$. For example, in (S1), $f^0$ is known, so we can solve $f^{(1,2)}$ on the left hand side first. After $f^{(1,2)}$ is known, it can be plugged into the right hand side of (S2) to solve for $f^{(1,1)}$, and so on. We have organized these equations such that the right hand side of an equation is known by solutions of equations above it, and the left hand side has only a single term with the unknown $f^{(i,j)}$ operated by $\mathcal{I}_c$, which is then solved by reversing $\mathcal{I}_c$.

This structure is general. At $E^2$ order, we obtain the following five equations for $f^{(2,j)}$ $(j=0,\cdots,4)$:

$$\hat{\mathcal{I}}_{\rm c}^{(0,-2)} f^{(2,4)} = \hat{\mathcal{D}}_{\rm E} f^{(1,2)}, \tag{S6}$$

$$\hat{\mathcal{I}}_{\rm c}^{(0,-2)} f^{(2,3)} = \hat{\mathcal{D}}_{\rm E} f^{(1,1)} - \hat{\mathcal{I}}_{\rm sk}^{(0,-3)} f^{(2,4)}, \tag{S7}$$

* xiaoziche@gmail.com

† yangshengyuan@um.edu.mo

‡ xiao.li@cityu.edu.hk

$$\hat{\mathcal{I}}_{\rm c}^{(0,-2)}\{f^{(2,2)}\} = \hat{\mathcal{D}}_{\rm E} f^{(1,0)} - \hat{\mathcal{I}}_{\rm sj}^{(1,-2)} f^{(1,2)} - \hat{\mathcal{I}}_{\rm sk}^{(0,-3)} f^{(2,3)} - \hat{\mathcal{I}}_{\rm sk}^{(0,-4)} f^{(2,4)}, \tag{S8}$$

$$\hat{\mathcal{I}}_{\rm c}^{(0,-2)} f^{(2,1)} = \hat{\mathcal{D}}_{\rm E} f^{(1,\text{-}1)} - \hat{\mathcal{I}}_{\rm sj}^{(1,-2)} f^{(1,1)} - \hat{\mathcal{I}}_{\rm sk}^{(1,-3)} f^{(1,2)} - \hat{\mathcal{I}}_{\rm sk}^{(0,-3)} f^{(2,2)} - \hat{\mathcal{I}}_{\rm sk}^{(0,-4)} f^{(2,3)}, \tag{S9}$$

$$\hat{\mathcal{I}}_{\rm c}^{(0,-2)} f^{(2,0)} = \hat{\mathcal{D}}_{\rm E} f^{(1,\text{-}2)} - \hat{\mathcal{I}}_{\rm sj}^{(1,-2)} f^{(1,0)} - \hat{\mathcal{I}}_{\rm sk}^{(1,-3)} f^{(1,1)} - \hat{\mathcal{I}}_{\rm sk}^{(1,-4)} f^{(1,2)} - \hat{\mathcal{I}}_{\rm sj}^{(2,-2)} f_0 - \hat{\mathcal{I}}_{\rm sk}^{(0,-3)} f^{(2,1)} - \hat{\mathcal{I}}_{\rm sk}^{(0,-4)} f^{(2,2)}. \tag{S10}$$

In these equations, the involved collision integrals are given by [1, 4]

$$\begin{aligned} &\hat{\mathcal{I}}_{\rm c}^{(0,-2)} f_l \equiv -\sum_{l'} \omega_{l'l}^{(2)} (f_l - f_{l'}), \quad \hat{\mathcal{I}}_{\rm sj}^{(1,-2)} f_l \equiv -\sum_{l'} \delta^E \omega_{l'l}^{(2)} (f_l - f_{l'}), \quad \hat{\mathcal{I}}_{\rm sj}^{(2,-2)} f_l \equiv -\sum_{l'} \delta^{E^2} \omega_{l'l}^{(2)} (f_l - f_{l'}), \\ &\hat{\mathcal{I}}_{\rm sk}^{(0,-3)} f_l \equiv -\sum_{l'} \omega_{l'l}^{(3a)} (f_l + f_{l'}), \quad \hat{\mathcal{I}}_{\rm sk}^{(0,-4)} f_l \equiv -\sum_{l'} \omega_{l'l}^{(4a)} (f_l + f_{l'}), \quad \hat{\mathcal{I}}_{\rm sk}^{(1,-4)} f_l \equiv -\sum_{l'} \delta^E \omega_{l'l}^{(4a)} (f_l + f_{l'}). \end{aligned} \tag{S11}$$

Here, the symbol $\delta^E$ ($\delta^{E^2}$) denotes the correction of the corresponding scattering kernel at $E$ ($E^2$) order. Here, $\omega_{l'l}^{(2)}$ and $\omega_{l'l}^{a}$ are the symmetric and antisymmetric scattering rate between $l$ and $l'$ states, respectively. Assuming weak disorders, it is sufficient to evaluate the symmetric scattering rate in the lowest Born order [5]. Nevertheless, to capture key features from skew scattering requires to retain $\omega_{l'l}^{a}$ at the third ($3a$) and fourth ($4a$) order in the disorder strength $V$ [3], i.e., $\omega_{ll'}^{a} \approx \omega_{ll'}^{(3a)} + \omega_{ll'}^{(4a)}$. Higher order processes do not bring in new scaling behavior, but merely renormalize the above terms.

In the analysis below, we will not just derive the scaling law for the nonlinear conductivity tensor $\chi_{abc}$. In addition, we will clarify the physical mechanisms that contribute to the ZOE terms. For this purpose, a convenient way is to track the extrinsic origin and scaling behavior of each contribution to $f^{(i,j)}$ and find which kind of collision integrals it comes from. For example, the conventional collision integral (the dominant one in $\hat{\mathcal{I}}$) scales with the longitudinal resistivity, i.e., $\hat{\mathcal{I}}_c \sim \rho_{xx}$, which gives, by (S1), $f^{(1,2)} \sim 1/\rho_{xx}$. When combined with the band group velocity, this gives the scaling of familiar linear longitudinal transport. The scaling forms of higher-rank $f^{(i,j)}$ can be derived similarly. For $f^{(1,0)}$, it has two contributions: one from side jump $\hat{\mathcal{I}}_{\rm sj}$ and one from intrinsic skew scattering $\hat{\mathcal{I}}_{\rm sk}^{(0,-4)}$. To stress these origins, we write

$$f^{(1,0)} = f^{(1,0),\rm SJ} + f^{(1,0),\rm ISK}. \tag{S12}$$

Analyzing their scaling with partial resistivities, we find

$$f^{(1,0),\rm SJ} \sim \rho_i/\rho_{xx}, \qquad f^{(1,0),\rm ISK} \sim \rho_i\rho_j/\rho_{xx}^2. \tag{S13}$$

Here, we used a simple notation, i.e., $\sim \rho_i/\rho_{xx}$ means that the quantity scales as $\sum_i \alpha_i \rho_i/\rho_{xx}$ (with coefficients $\alpha_i$ independent of disorder concentration). The notation in the second expression is similar. Like in the linear anomalous Hall effect, the ZOE terms do not depend on the non-Gaussian disorder correlation $\omega^{(3a)}$. Hence, we first neglect $\omega^{(3a)}$ terms in studying the ZOE terms. The effect of non-Gaussian disorder correlation will be analyzed in a while. Then, we find the results for the relevant $f^{(i,j)}$ are

$$f^{(2,2)} = f^{(2,2),\rm SJ} + f^{(2,2),\rm ISK}, \qquad f^{(2,2),\rm SJ} \sim \rho_i/\rho_{xx}^2, \qquad f^{(2,2),\rm ISK} \sim \rho_i\rho_j/\rho_{xx}^3. \tag{S14}$$

$$f^{(2,0)} = f^{(2,0),\rm E-SJ} + f^{(2,0),\rm E-ISK} + f^{(2,0),\rm SJ-SJ} + f^{(2,0),\rm SJ-ISK} + f^{(2,0),\rm ISK-ISK}, \tag{S15}$$

where

$$f^{(2,0),\rm E-SJ} \sim \rho_i/\rho_{xx}, \qquad f^{(2,0),\rm E-ISK} \sim \rho_i\rho_j/\rho_{xx}^2, \qquad f^{(2,0),\rm SJ-SJ} \sim \rho_i\rho_j/\rho_{xx}^2, \tag{S16}$$

$$f^{(2,0),\rm SJ-ISK} \sim \rho_i\rho_j\rho_k/\rho_{xx}^3, \qquad f^{(2,0),\rm ISK-ISK} \sim \rho_i\rho_j\rho_k\rho_\ell/\rho_{xx}^4. \tag{S17}$$

Here, the superscript 'E-SJ' means that the contribution involves $E$ field corrected side jump collision integral, similar for 'E-ISK'; 'SJ-SJ' means that the contribution involves the side jump collision integral twice, similar for 'SJ-ISK' and 'ISK-ISK'.

The velocity of an electron wave packet has been given in Eq. (2) of the main text. Here, we simplify the notation and re-write it as

$$v = v^b + v^a + v^{\rm sj} + \delta^E v^{\rm sj}, \tag{S18}$$

where $v^b$ is the band velocity, $v^a$ is the anomalous velocity, and we explicitly separate out the field correction to side jump velocity as $\delta^E v^{\rm sj}$, so $v^{\rm sj}$ here denotes the side jump velocity without field correction. As mentioned in the main text, the first two terms are independent of scattering, whereas $v^{\rm sj}$ and $\delta^E v^{\rm sj}$ scales as $\sim \rho_i$.

Now, we can collect all terms in the result to find the zeroth order terms in nonlinear conductivity $\chi$. We find that the $\tau^0$-term $\chi^0$ consists of the following parts

$$\chi^0 = \chi^{\rm int} + \chi^{\rm A-SJ} + \chi^{\rm A-ISK} + \chi^{\rm E-SJ} + \chi^{\rm E-ISK} + \chi^{\rm SJ-SJ} + \chi^{\rm SJ-ISK} + \chi^{\rm ISK-ISK}, \tag{S19}$$

where $\chi^{\rm int}$ is the intrinsic contribution from Berry connection polarizability [6–8], and the other terms are ZOE effects. Specifically, their origin and scaling can be obtained as

$$\chi^{\rm A-SJ} : f^{(1,0),{\rm SJ}} v^a \sim \sum_i \mathfrak{c}_i^{\text{A-SJ}} \rho_i/\rho_{xx}, \qquad \chi^{\rm A-ISK} : f^{(1,0),{\rm ISK}} v^a \sim \sum_{ij} \mathfrak{c}_{ij}^{\text{A-ISK}} \rho_i\rho_j/\rho_{xx}^2. \tag{S20}$$

These two ZOE contributions are due to side jump (skew scattering) induced non-equilibrium distribution combined with anomalous velocity.

$$\chi^{\rm E-SJ} : f^{(2,0),{\rm E-SJ}} v^b + f^{(1,2)}\delta^E v^{\rm sj} \sim \sum_i \mathfrak{c}_i^{\text{E-SJ}} \rho_i/\rho_{xx}, \qquad \chi^{\rm E-ISK} : f^{(2,0),{\rm E-ISK}} v^b \sim \sum_{ij} \mathfrak{c}_{ij}^{\text{E-ISK}} \rho_i\rho_j/\rho_{xx}^2, \tag{S21}$$

which are due to field corrections to side jump (skew scattering) process.

$$\chi^{\rm SJ-SJ} : f^{(2,0),{\rm SJ-SJ}} v^b + f^{(2,2),{\rm SJ}} v^{\rm sj} \sim \sum_{ij} \mathfrak{c}_{ij}^{\text{SJ-SJ}} \rho_i\rho_j/\rho_{xx}^2, \qquad \chi^{\rm ISK-ISK} : f^{(2,0),{\rm ISK-ISK}} v^b \sim \sum_{ijk\ell} \mathfrak{c}_{ij}^{\text{ISK-ISK}} \rho_i\rho_j\rho_k\rho_\ell/\rho_{xx}^4, \tag{S22}$$

which involve two side jump (skew scattering) processes, and

$$\chi^{\rm SJ-ISK} : f^{(2,0),{\rm SJ-ISK}} v^b + f^{(2,2),{\rm ISK}} v^{\rm sj} \sim \sum_{ijk} \mathfrak{c}_{ijk}^{\text{SJ-ISK}} \rho_i\rho_j\rho_k/\rho_{xx}^3, \tag{S23}$$

which involves a side jump and a skew scattering. All the coefficients $\mathfrak{c}$ above are independent of disorder concentration.

Collecting all these terms, we find zeroth order terms in the scaling law Eq. (17) of the main text. Moreover, the above analysis gives the origin of each term. Specifically, we find the scaling coefficients in Eq. (17) are given by

$$c^{\rm int} = \mathfrak{c}^{\rm int}, \quad c_i = \mathfrak{c}_i^{\rm A-SJ} + \mathfrak{c}_i^{\rm E-SJ}, \quad c_{ij} = \mathfrak{c}_{ij}^{\rm A-ISK} + \mathfrak{c}_{ij}^{\rm E-ISK} + \mathfrak{c}_{ij}^{\rm SJ-SJ}, \quad c_{ijk} = \mathfrak{c}_{ijk}^{\rm SJ-ISK}, \quad c_{ijk\ell} = \mathfrak{c}_{ijk\ell}^{\rm ISK-ISK}. \tag{S24}$$

Next, we add back the non-Gaussian disorder correlation, i.e., the skew scattering part $\omega^{(3a)}$. As discussed in the main text, it comes only from static disorders and does not contribute to ZOE terms. Its main effect in $\mathcal{T}$-odd nonlinear transport is through the induced $f^{(2,1)}$ term, which scales as

$$f^{(2,1)} \sim \sum_{i\in S} \frac{\rho_i}{\rho_{xx}^2}(\mathfrak{d}_i + \sum_j \mathfrak{d}_{ij}\frac{\rho_j}{\rho_{xx}} + \sum_{jk}\mathfrak{d}_{ijk}\frac{\rho_j\rho_k}{\rho_{xx}^2} + \sum_{j\in S}\mathfrak{d}_{ij}\frac{\rho_j}{\rho_{xx}^2}). \tag{S25}$$

Combined with the band velocity, this gives the scaling terms with $d$ and $\mathcal{D}$ coefficients in Eq. (6) of main text. Finally, adding in the Drude-like term at $\tau^2$ order, we arrive at the scaling law Eq. (6) for $\mathcal{T}$-odd nonlinear transport:

$$\begin{aligned}\chi_{yxx} = c^{\rm int} &+ \sum_i c_i \frac{\rho_i}{\rho_{xx}} + \sum_{i,j} c_{ij}\frac{\rho_i\rho_j}{\rho_{xx}^2} + \sum_{ijk} c_{ijk}\frac{\rho_i\rho_j\rho_k}{\rho_{xx}^3} + \sum_{ijk\ell} c_{ijk\ell}\frac{\rho_i\rho_j\rho_k\rho_\ell}{\rho_{xx}^4} \\ &+ \sum_{i\in S}\frac{\rho_i}{\rho_{xx}^2}(d_i + \sum_j d_{ij}\frac{\rho_j}{\rho_{xx}} + \sum_{jk} d_{ijk}\frac{\rho_j\rho_k}{\rho_{xx}^2} + \sum_{j\in S}\mathcal{D}_{ij}\frac{\rho_j}{\rho_{xx}^2}) + D\frac{1}{\rho_{xx}^2}.\end{aligned} \tag{S26}$$

As a most encountered example, we consider two major scattering sources: one temperature independent ($i = 0$), and one temperature dependent ($i = 1$), usually impurity and phonon, respectively [9]. Then the scaling in terms of conductivities becomes [Eq. (9) in the main text]

$$\chi_{yxx} = \lambda_0 + \lambda_1\frac{\sigma}{\sigma_0} + \lambda_2\frac{\sigma^2}{\sigma_0^2} + \lambda_3\frac{\sigma^3}{\sigma_0^3} + \lambda_4\frac{\sigma^4}{\sigma_0^4} + \eta_2\frac{\sigma^2}{\sigma_0} + \eta_3\frac{\sigma^3}{\sigma_0^2} + \eta_4\frac{\sigma^4}{\sigma_0^3} + \gamma_4\frac{\sigma^4}{\sigma_0^2} + D\sigma^2, \tag{S27}$$

where the scaling parameters are given by

$$\begin{aligned}
\lambda_0 =& c^{\text{int}} + c_1 + c_{11} + c_{111} + c_{1111},\\
\lambda_1 =& c_0 - c_1 + 2(c_{01} - c_{11}) + 3(c_{011} - c_{111}) + 4(c_{0111} - c_{1111}),\\
\lambda_2 =& c_{00} - 2c_{01} + c_{11} + 3(c_{001} - 2c_{011} + c_{111}) + 6(c_{0011} - 2c_{0111} + c_{1111}),\\
\lambda_3 =& c_{000} - 3c_{001} + 3c_{011} - c_{111} + 4(c_{0001} - 3c_{0011} + 3c_{0111} - c_{1111}),\\
\lambda_4 =& c_{0000} - 4c_{0001} + 6c_{0011} - 4c_{0111} + c_{1111},\\
\eta_2 =& d_0 + d_{01} + d_{011},\\
\eta_3 =& d_{00} - d_{01} + 2(d_{001} - d_{011}),\\
\eta_4 =& d_{000} - 2d_{001} + d_{011},\\
\gamma_4 =& \mathcal{D}_{00}.
\end{aligned} \tag{S28}$$

All the $\eta$'s and $\gamma_4$ are related to the conventional third order skew scattering.

As the above scaling analysis holds for both transverse and longitudinal nonlinear transport, the scaling for longitudinal nonlinear conductivity $\chi_{xxx}$ takes the same form as transverse transport, except that there is no intrinsic contribution [6–8, 10].

## II. SOLUTION OF ZOE TERMS FROM BOLTZMANN EQUATION

In the section above, we derive the general scaling law. Now, if one is given a specific disorder model, the ZOE terms can also be explicitly calculated by using our Boltzmann equation approach. In the following we assume a single type of disorder without non-Gaussian correlation to obtain the scaling parameters in the zeroth-order term in Table. I of the main text. Specifically,

$$f_l^{(1,0),\text{SJ}} = -\tau E_a \sum_{l'} \left[\Xi_{ll',a}\delta(\varepsilon_l - \varepsilon_{l'}) + O_{ll',a}\right]\left(f_l^0 - f_{l'}^0\right) = -\tau E_a \sum_{l'} O_{ll',a}\left(f_l^0 - f_{l'}^0\right), \tag{S29}$$

$$f_l^{(1,0),\text{ISK}} = -\tau^2 \boldsymbol{E}\cdot\sum_{l'} \omega_{l'l}^{(4a)}(\partial_{\boldsymbol{k}} f_l^0 + \partial_{\boldsymbol{k}'} f_{l'}^0), \tag{S30}$$

$$\begin{aligned}
f_l^{(2,2),\text{SJ}} =& -\tau^2 E_a E_b \partial_a \sum_{l'} \left[\Xi_{ll',b}\delta(\varepsilon_l - \varepsilon_{l'}) + O_{ll',b}\right]\left(f_l^0 - f_{l'}^0\right)\\
& -\tau^2 E_a E_b \sum_{l'} \left[\Xi_{ll',a}\delta(\varepsilon_l - \varepsilon_{l'}) + O_{ll',a}\right](\partial_b f_l^0 - \partial_{b'} f_{l'}^0),
\end{aligned} \tag{S31}$$

$$f_l^{(2,0),\text{E}-\text{SJ}} = \tau E_a E_b \sum_{l'} Q_{ll'}^{ab} \frac{\partial\delta(\varepsilon_l - \varepsilon_{l'})}{\partial\varepsilon_l}\left(f_l^0 - f_{l'}^0\right) - \frac{1}{2}\tau E_a E_b \sum_{l'} P_{ll'}^{ab}\left(f_l^0 - f_{l'}^0\right), \tag{S32}$$

$$f_l^{(2,0),\text{SJ}-\text{SJ}} = -\tau \sum_{l'} [\Xi_{ll',b}\delta(\varepsilon_l - \varepsilon_{l'}) + O_{ll',b}] E_b [f_l^{(1,0),\text{SJ}} - f_{l'}^{(1,0),\text{SJ}}], \tag{S33}$$

$$f_l^{(2,0),\text{SJ}-\text{ISK}} = -\tau \sum_{l'} [\Xi_{ll',b}\delta(\varepsilon_l - \varepsilon_{l'}) + O_{ll',b}] E_b [f_l^{(1,0),\text{ISK}} - f_{l'}^{(1,0),\text{ISK}}] - \tau \sum_{l'} \omega_{l'l}^{(4a)} [f_l^{(2,2),\text{SJ}} + f_{l'}^{(2,2),\text{SJ}}], \tag{S34}$$

$$f_l^{(2,2),\text{ISK}} = \tau \boldsymbol{E}\cdot\partial_{\boldsymbol{k}} f_l^{(1,0),\text{ISK}} - \tau \sum_{l'} \omega_{l'l}^{(4a)} \left[(\tau\boldsymbol{E}\cdot\partial_{\boldsymbol{k}})^2 f_l^0 + (\tau\mathbf{E}\cdot\partial_{\boldsymbol{k}'})^2 f_{l'}^0\right], \tag{S35}$$

$$f_l^{(2,0),\text{E}-\text{ISK}} = -\tau^2 \boldsymbol{E}\cdot\sum_{l'} (\boldsymbol{K}_{l'l}^{\text{ISK}}\cdot\boldsymbol{E})(\partial_{\boldsymbol{k}} f_l^0 + \partial_{\boldsymbol{k}'} f_{l'}^0), \tag{S36}$$

$$f_l^{(2,0),\mathrm{ISK-ISK}} = -\tau \sum_{l'} \omega_{l'l}^{(4a)} \left[ f_l^{(2,2),\mathrm{ISK}} + f_{l'}^{(2,2),\mathrm{ISK}} \right]. \tag{S37}$$

In these equations,

$$\Xi_{ll',a} = 4\pi \,\mathrm{Re} \left( \sum_{m\neq l'} \frac{\langle u_m | i\partial_a u_{l'} \rangle \langle V_{l'l} V_{lm} \rangle_c}{\varepsilon_{l'} - \varepsilon_m} + \sum_{m \neq l} \frac{\langle V_{ll'} V_{l'm} \rangle_c \langle u_m | i\partial_a u_l \rangle}{\varepsilon_l - \varepsilon_m} \right) \tag{S38}$$

and

$$O_{ll',a} = 2\pi \langle |V_{ll'}|^2 \rangle_c \delta r_{ll',a} \frac{\partial \delta(\varepsilon_l - \varepsilon_{l'})}{\partial \varepsilon_l} \tag{S39}$$

are from the side jump collision integral [1]

$$\hat{\mathcal{I}}_{\mathrm{sj}}^{(1,-2)} f_l = - E_a \sum_{l'} \left[ \Xi_{ll',a} \delta(\varepsilon_l - \varepsilon_{l'}) + O_{ll',a} \right] (f_l - f_{l'}). \tag{S40}$$

Here, $\langle \cdots \rangle_c$ denotes the average over disorder configuration, and $V_{ll'}$ the scattering matrix element. In the model calculation, we take the white-noise pointlike disorder, with $n_i$ the disorder concentration. The field effects in scattering (i.e., side jump) consist of both the electrical work done due to coordinate shift and field induced change of scattering amplitude through interband mixing [1]. In (S39),

$$\delta r_{l'l,a} = \langle u_{l'} | i\partial_{a'} u_{l'} \rangle - \langle u_l | i\partial_a u_l \rangle - (\partial_a + \partial_{a'}) \arg V_{l'l}, \tag{S41}$$

with $\partial_{a'} \equiv \partial_{k'_a}$, is the coordinate shift appearing in side jump velocity

$$v_a^{\mathrm{sj}} = 2\pi \sum_{l'} \langle |V_{ll'}|^2 \rangle_c \delta r_{l'l,a} \delta(\varepsilon_l - \varepsilon_{l'}) = \sum_{l'} \delta R_{ll',a} \delta(\varepsilon_l - \varepsilon_{l'}), \tag{S42}$$

where in the second step [11] we defined

$$\delta R_{ll',a} := 2\pi \,\mathrm{Re}[\sum_{m\neq l} \langle V_{ml'} V_{l'l} \rangle_c \langle u_l | i\partial_a u_m \rangle - (l \leftrightarrow l')]. \tag{S43}$$

Moreover,

$$\begin{aligned} Q_{ll'}^{ab} = 2\pi n_i V_0^2 \,\mathrm{Re} \sum_{p\neq l} \Big[ & \sum_{q\neq p} \frac{\langle i\partial_b u_p | u_q \rangle \langle u_q | u_{l'} \rangle \langle u_{l'} | u_l \rangle \langle u_l | i\partial_a u_p \rangle}{\varepsilon_p - \varepsilon_q} \\ & + \sum_{q\neq l'} \frac{\langle u_p | u_q \rangle \langle u_q | i\partial_b u_{l'} \rangle \langle u_{l'} | u_l \rangle \langle u_l | i\partial_a u_p \rangle}{\varepsilon_{l'} - \varepsilon_q} + \sum_{q\neq l'} \frac{\langle u_p | u_{l'} \rangle \langle i\partial_b u_{l'} | u_q \rangle \langle u_q | u_l \rangle \langle u_l | i\partial_a u_p \rangle}{\varepsilon_{l'} - \varepsilon_q} \\ & + \sum_{q\neq l} \frac{\langle u_p | u_{l'} \rangle \langle u_{l'} | u_q \rangle \langle u_q | i\partial_b u_l \rangle \langle u_l | i\partial_a u_p \rangle}{\varepsilon_l - \varepsilon_q} + \sum_{q\neq l} \frac{\langle u_p | u_{l'} \rangle \langle u_{l'} | u_l \rangle \langle i\partial_b u_l | u_q \rangle \langle u_q | i\partial_a u_p \rangle}{\varepsilon_l - \varepsilon_q} \\ & + \sum_{q\neq p} \frac{\langle u_p | u_{l'} \rangle \langle u_{l'} | u_l \rangle \langle u_l | i\partial_b u_q \rangle \langle u_q | i\partial_a u_p \rangle}{\varepsilon_p - \varepsilon_q} + \sum_{q\neq p} \frac{\langle u_p | u_{l'} \rangle \langle u_{l'} | u_l \rangle \langle u_l | u_q \rangle \, i\partial_b \langle u_q | i\partial_a u_p \rangle}{\varepsilon_p - \varepsilon_q} \\ & - (l \leftrightarrow l') \Big] \end{aligned} \tag{S44}$$

and

$$P_{ll'}^{ab} = -\delta R_{ll',a} \delta r_{ll',b} \frac{\partial^2 \delta(\varepsilon_l - \varepsilon_{l'})}{\partial \varepsilon_l^2} \tag{S45}$$

are from the $E$-field corrected side jump collision integral

$$\hat{\mathcal{I}}_{\mathrm{sj}}^{(2,-2)} f_l^0 = E_a E_b \sum_{l'} Q_{ll'}^{ab} \frac{\partial \delta(\varepsilon_l - \varepsilon_{l'})}{\partial \varepsilon_l} (f_l^0 - f_{l'}^0) - \frac{1}{2} E_a E_b \sum_{l'} P_{ll'}^{ab} (f_l^0 - f_{l'}^0). \tag{S46}$$

Lastly, $K^{\rm ISK}_{l'l}$ measures $E$-field induced correction to $\omega^{(4a)}_{l'l}$, i.e., we defined $\delta^E\omega^{(4a)}_{l'l} = K^{\rm ISK}_{l'l,a}E_a$.

The field correction of side-jump velocity is then given by

$$\delta^E v^{\rm sj}_{l,a} = \sum_{l'}\Big[\delta R_{ll',a}\frac{\partial\delta(\varepsilon_l-\varepsilon_{l'})}{\partial\varepsilon_l}\delta r_{ll',b}E_b + Q^{ab}_{ll'}\delta(\varepsilon_l-\varepsilon_{l'})E_b\Big]. \tag{S47}$$

With the above ingredients, the ZOE terms in nonlinear conductivity can be solved out for a specific model, such as the Dirac model discussed in the main text. To help identify the order of disorder in various contributions, one notes that in the presence of a single type of scattering source, $\frac{1}{\tau}\sim O_{ll'}\sim\omega^{(2)}_{ll'}\sim\delta R\sim Q\sim\Xi\sim v^{\rm sj}$, and $\frac{1}{\tau^2}\sim\omega^{(4a)}_{ll'}\sim K^{\rm Isk}_{ll'}$. In addition, in the following expressions, we add back the electric charge $e$ and $\hbar$.

Label this disorder by $i=1$. In our notation, we have $c_1 = \chi^{\rm A-SJ}+\chi^{\rm E-SJ}$, and

$$\chi^{\rm A-SJ}_{abc} = \varepsilon_{abd}\frac{e^3\tau}{\hbar}\sum_l \Omega_{l,d}v^{\rm sj}_{l,c}(f^0)', \tag{S48}$$

$$\begin{aligned}\chi^{\rm E-SJ}_{abc} =& -e^2\tau\sum_{l,l'}\left(Q^{ac}_{ll'}v_{l,b} - Q^{bc}_{ll'}v_{l,a}\right)\delta(\varepsilon_l-\varepsilon_{l'})(f^0)' &\text{(S49)}\\ &+e^3\tau\sum_{l,l'}\Big\{-\partial_a\left[\delta R_{ll',b}\delta r_{ll',c}\delta(\varepsilon_l-\varepsilon_{l'})\right] - \partial_c\left[\delta R_{ll',a}\delta r_{ll',b}\delta(\varepsilon_l-\varepsilon_{l'})\right]\Big\}(f^0)'\\ &+e^3\tau\sum_{l,l'}\Big\{\partial_c\left[\delta R_{ll',a}\delta r_{ll',b}\right]\delta(\varepsilon_l-\varepsilon_{l'}) + \frac{1}{2}\partial_a\left[\delta R_{ll',b}\delta r_{ll',c}\right]\delta(\varepsilon_l-\varepsilon_{l'})\Big\}(f^0)', &\text{(S50)}\end{aligned}$$

with $(f^0)'\equiv\partial_{\varepsilon_l}f_0$.

Second, $c_{11} = \chi^{\rm A-ISK}+\chi^{\rm E-ISK}+\chi^{\rm SJ-SJ}$, where

$$\chi^{\rm A-ISK}_{abc} = \varepsilon_{abd}\frac{e^3\tau^2}{\hbar^2}\sum_{l,l'}\left(\Omega_{l,d}-\Omega_{l',d}\right)\omega^{\rm (4a)}_{l'l}\partial_c f^0, \tag{S51}$$

$$\chi^{\rm E-ISK}_{abc} = e^2\tau^2\sum_{l,l'}\left(v_{l,a}-v_{l,a}\right)v_{l,b}K^{\rm ISK}_{l'l,c}(f^0)', \tag{S52}$$

$$\begin{aligned}\chi^{\rm SJ-SJ}_{abc} =& \frac{e^3\tau^2}{\hbar}\sum_l\Big[-\partial_b v^{\rm sj}_{l,a}v^{\rm sj}_{l,c} - \sum_{l'}(v^{\rm sj}_{l,a}-v^{\rm sj}_{l',a})\delta R_{ll',c}\partial_b\delta(\varepsilon_l-\varepsilon_{l'}) + \sum_{l'}(v^{\rm sj}_{l,a}-v^{\rm sj}_{l',a})\Xi_{ll',c}v_{l,b}\delta(\varepsilon_l-\varepsilon_{l'})\Big](f^0)'\\ &+e^2\tau^2\sum_{l,l'}\left(v_{l,a}-v_{l',a}\right)\left[\Xi_{ll',b}\delta(\varepsilon_l-\varepsilon_{l'})+O_{ll',b}\right]v^{\rm sj}_{l,c}(f^0)'. &\text{(S53)}\end{aligned}$$

Third, $c_{111} = \chi^{\rm SJ-ISK}$, where

$$\begin{aligned}\chi^{\rm SJ-ISK}_{abc} =& \frac{e^3\tau^3}{\hbar^2}\sum_{l,l'}\Big[(\partial_{b'}v^{\rm sj}_{l',a}-\partial_b v^{\rm sj}_{l,a})\omega^{(4a)}_{l'l}\partial_c f^0 + (v^{\rm sj}_{l,a}-v^{\rm sj}_{l',a})\omega^{(4a)}_{l'l}\partial_b\partial_c f^0\Big]\\ &-\frac{e^2\tau^3}{\hbar}\sum_{l,l',l''}\Big[\left(v_{l,a}-v_{l',a}\right)\left[\Xi_{ll',b}\delta(\varepsilon_l-\varepsilon_{l'})+O_{ll',b}\right] - \left(v_{l'',a}-v_{l',a}\right)\left[\Xi_{l''l',b}\delta(\varepsilon_{l''}-\varepsilon_{l'})+O_{l''l',b}\right]\Big]\omega^{(4a)}_{l''l}\partial_c f^0\\ &+\frac{e^3\tau^3}{\hbar}\sum_{l,l'}\partial_b(v_{l,a}\omega^{(4a)}_{l'l}-v_{l',a}\omega^{(4a)}_{l'l})v^{\rm sj}_{l,c}(f^0)'\\ &-\frac{e^2\tau^3}{\hbar}\sum_{l,l',l''}\Big[(v_{l,a}-v_{l',a})\omega^{(4a)}_{l'l} - (v_{l'',a}-v_{l',a})\omega^{(4a)}_{l'l''}\Big]\Big[\Xi_{ll'',c}\delta(\varepsilon_l-\varepsilon_{l''})+O_{ll'',c}\Big]\partial_b f^0. &\text{(S54)}\end{aligned}$$

Fourth, $c_{1111} = \chi^{\rm ISK-ISK}$, where

$$\chi^{\rm ISK-ISK}_{abc} = \frac{e^3\tau^4}{\hbar}\sum_{l,l',l''}\Big\{\Big(\partial_b[(v_{l,a}-v_{l',a})\omega^{(4a)}_{l'l}]\omega^{(4a)}_{l''l} + \partial_b\Big[(v_{l,a}-v_{l',a})\omega^{(4a)}_{l'l}\omega^{(4a)}_{l''l}\Big]\Big) + (l\leftrightarrow l'')\Big\}\partial_c f^0. \tag{S55}$$

The above formulas are used to calculate the ZOE contributions for the Dirac model in the main text.

## III. TRANSVERSE ZOE CONDUCTIVITIES IN DIRAC MODEL

As mentioned in the main text, the transverse nonlinear conductivity $\chi_{yxx}$ can be separated into two parts according to the symmetry of the first two indices: $\chi_{yxx} = \chi_{[yx]x} + \chi_{(yx)x}$, where the square (round) bracket means antisymmetrization (symmetrization) of indices. The antisymmetric part is dissipationless, whereas the symmetric part is dissipative. For the Dirac model studied in the main text, both parts exist and have comparable magnitudes. The intrinsic term is dissipationless, so it appears only in $\chi_{[yx]x}$. The calculation results for the two parts are shown in Fig. S1.

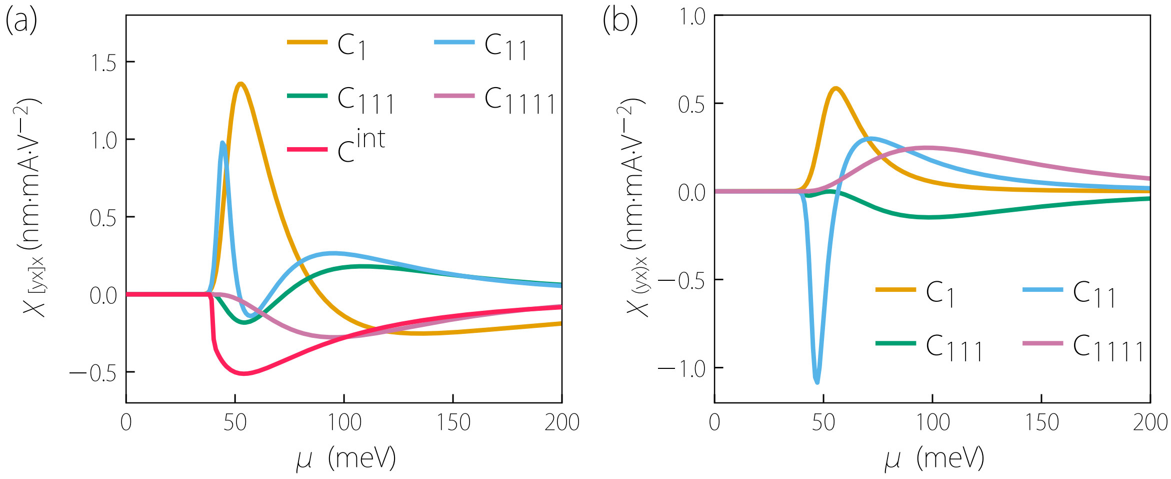


FIG. S1. Contributions to the zeroth order term in (a) $\chi_{[yx]x} = (\chi_{yxx} - \chi_{xyx})/2$ and (b) $\chi_{(yx)x} = (\chi_{yxx} + \chi_{xyx})/2$ for the Dirac model in main text. The parameters are: $v = 1 \times 10^6$ m/s, $\Delta = 40$ meV, and $w/v = 0.2$.


[1] C. Xiao, Z. Z. Du, and Q. Niu, Phys. Rev. B **100**, 165422 (2019).
[2] N. A. Sinitsyn, A. H. MacDonald, T. Jungwirth, V. K. Dugaev, and J. Sinova, Phys. Rev. B **75**, 045315 (2007).
[3] N. A. Sinitsyn, J. Phys.: Condens. Matter **20**, 023201 (2007).
[4] Z. Z. Du, C. M. Wang, S. Li, H.-Z. Lu, and X. C. Xie, Nat. Commun. **10**, 3047 (2019).
[5] N. Nagaosa, J. Sinova, S. Onoda, A. H. MacDonald, and N. P. Ong, Rev. Mod. Phys. **82**, 1539 (2010).
[6] Y. Gao, S. A. Yang, and Q. Niu, Phys. Rev. Lett. **112**, 166601 (2014).
[7] C. Wang, Y. Gao, and D. Xiao, Phys. Rev. Lett. **127**, 277201 (2021).
[8] H. Liu, J. Zhao, Y.-X. Huang, W. Wu, X.-L. Sheng, C. Xiao, and S. A. Yang, Phys. Rev. Lett. **127**, 277202 (2021).
[9] D. Hou, G. Su, Y. Tian, X. Jin, S. A. Yang, and Q. Niu, Phys. Rev. Lett. **114**, 217203 (2015).
[10] C. Xiao, J. Cao, Q. Niu, and S. A. Yang, arXiv:2406.11180.
[11] C. Xiao and Q. Niu, Phys. Rev. B **96**, 045428 (2017).
